# Supplementary material for: Software Verification with CPAchecker 3.0: Tutorial and User Guide (Extended Version)
Source: arXiv:2409.02094 source file (2024-09-03)
Supplement: Supplementary file 1 [file configuration.tex]

\section{Configuring Composite CPA}
\label{appendix:compositeCPA}

\cpachecker contains implementation of various CPAs
(please refer to \cref{sec:cpa-concept} for the high-level explanation of CPA concept),
including
\texttt{ARGCPA} that monitors the explored abstract reachability graph,
\texttt{LocationCPA} that keeps track of explicit program locations,
\texttt{PredicateCPA} that encodes program paths into SMT formulas,
\texttt{LoopBoundCPA} that counts the number of visits to a loop head on a program path, and
\texttt{ValueAnalysisCPA} that records the concrete values of program variables at each location.
There are also other helper CPAs for some specific analyses,
for instance,
\texttt{OverflowCPA} is used for overflow detection (cf. \cref{sec:overflow})
to encode overflow conditions as errors internally in \cpachecker, and
\texttt{TestTargetCPA} is used for test-case generation (cf. \cref{sec:test-gen})
to indicate the locations of test goals.
Multiple CPAs can be combined as a \texttt{CompositeCPA}.
More information is available in \cpachecker's documentation
\href{https://svn.sosy-lab.org/software/cpachecker/tags/cpachecker-3.0/doc/Configuration.md#specifying-the-cpas}{doc/Configuration.md}.

In the following, we demonstrate how to create your own configuration for test-case generation.
% Also, you may configure our own analysis.
We recommend you to start with adapting an existing verification configuration.
Since you want to extract test cases from counterexamples,
the configuration should be able to record the explored state space in an abstract reachability graph,
that is, \texttt{ARGCPA} should be used.
To track test goals, you also need to add the \texttt{TestTargetCPA} to the analysis configuration,
as, e.g., has been done as follows in our example configuration.
\begin{Verbatim}[breaklines=true]
cpa               = cpa.arg.ARGCPA
ARGCPA            = cpa.composite.CompositeCPA
CompositeCPA.cpas = cpa.location.LocationCPA, cpa.callstack.CallstackCPA, cpa.functionpointer.FunctionPointerCPA, cpa.predicate.PredicateCPA, cpa.testtargets.TestTargetCPA
\end{Verbatim}
Note that \texttt{ARGCPA} has to be the top-level wrapper CPA that wraps \texttt{CompositeCPA},
which then wraps the remaining CPAs.
Additionally, you need to configure \cpachecker to construct test cases by enabling the option
\texttt{analysis.useTestCaseGeneratorAlgorithm}.
To enable test-case export of violations detected during verification, you need to enable the option~\texttt{counterexample.export.\-exportTestCase} and specify the desired test case format as discussed in \cref{sec:test-gen}.
% Note that the export only works if the analysis supports counterexample export, i.e., uses an \texttt{ARGCPA}.
